# Supplementary material for: UMO: Unified In-Context Learning Unlocks Motion Foundation Model Priors
Source: arXiv:2603.15975 source file (2026-03-16)
Supplement: Supplementary file 1 [file reaction_generation_supp.tex]

\begin{table}[t]
    \centering
    \caption{\textbf{Full Reaction Generation Results on Inter-X.} $\uparrow$ indicates higher is better, $\downarrow$ indicates lower is better, $\rightarrow$ indicates closer to ground truth is better. \textbf{Bold} indicates best, \underline{underline} indicates second best.}
    \label{tab:reaction_generation_supp}
    \footnotesize
    \setlength{\tabcolsep}{5pt}
    
    \begin{tabular}{lcccccc}
    \toprule
    Methods & FID $\downarrow$ & R@1 $\uparrow$ & R@2 $\uparrow$ & R@3 $\uparrow$ & MM-D $\downarrow$ & Div $\rightarrow$ \\
    \midrule
    Real & 0.002 & 0.429 & 0.626 & 0.736 & 3.536 & 9.734 \\
    \midrule
    \multicolumn{7}{c}{\textcolor{gray}{\textit{Baselines}}} \\
    TEMOS & 29.258 & 0.092 & 0.171 & 0.238 & 6.867 & 4.738 \\
    T2M & 5.481 & 0.184 & 0.298 & 0.396 & 9.576 & 5.771 \\
    MDM & 23.701 & 0.203 & 0.329 & 0.426 & 9.548 & 5.856 \\
    MDM (GRU) & 32.617 & 0.179 & 0.299 & 0.387 & 9.557 & 7.003 \\
    ComMDM & 29.266 & 0.090 & 0.165 & 0.236 & 6.870 & 4.734 \\
    InterGen & 5.207 & 0.207 & 0.335 & 0.429 & 9.580 & 7.788 \\
    InterMask & 0.399 & 0.403 & 0.595 & 0.705 & 3.705 & 9.046 \\
    \midrule
    \multicolumn{7}{c}{\textcolor{gray}{\textit{\method}}} \\
    \method & \textbf{xx} & \textbf{xx} & \textbf{xx} & \textbf{xx} & \textbf{xx} & xx \\
    \bottomrule
    \end{tabular}
\end{table}
